# Supplementary material for: Verification of Relational Data-Centric Dynamic Systems with External Services
Source: arXiv:1203.0024 source file (2012-02-29)
Supplement: Supplementary file 1 [file appendix-det-abstract.tex]

\subsection{History Preserving Bisimulation Result}

Consider a \dcds $\S = \tup{\dl,\pl}$ with data layer $\dl =
\tup{\CONST,\schema,\EC,\idb}$ and process layer
$\pl=\tup{\FUNC,\aset,\rset}$. Let $\cts{\sys} =
\tup{\CONST,\schema,\Sigma_c,s^0_s,\db_c,\Longrightarrow_c}$ and $\sts{\sys} =
\tup{\HERBRAND,\schema,\Sigma_s,s^0_s,\db_s,\Longrightarrow_s}$ be the
concrete and runtime transition systems of $\S$ built following the
deterministic services semantics. 

In order to prove that the symbolic and the concrete transition
systems are history preserving bisimilar, we define a notion of
\emph{compatibility} between their states, and then show that
compatibility implies history preserving bisimilarity.

To this end, we need to extend the service call maps contained in the
concrete states by also taking into account the constants of the
initial active domain $\adom{\idb}$. In particular, given a \cstate
$s_c = \tup{\I_c,\rmap} \in \Sigma_c$, we introduce $\rmapext$ as the extension
of $\rmap$ that maps each constant of the initial active domain to itself. Formally,
$\rmapext: \domain{\rmap} \cup \adom{\idb} \longrightarrow \CONST$,
and:
\begin{itemize}
\item for every term $t \in \domain{\rmap}$, $\rmapext(t) =
\rmap(t)$;
\item for every constant $c \in \adom{\idb}$, $\rmapext(c)
= c$.
\end{itemize}

We say that a \cstate $s_c = \tup{\I_c,\rmap} \in \Sigma_c$ is
\emph{compatible} with an \sstate $s_s = \tup{\I_s,\history} \in
\Sigma_s$ if there exists a bijection $\bcomp: \terms{\history}
\longrightarrow \domain{\rmapext}$ such that: 
\begin{enumerate}
\item for each value $d \in \adom{\idb}$, $\bcomp(d) = d$;
\item for each term $f(t_1,\ldots,t_n) \in \terms{\history}$,
  $\bcomp(f(t_1,\ldots,t_n)) = f(d_1,\ldots,d_n)$, where $d_i =
  \rmapext(\bcomp(t_i))$ for each $i \in \{1,\ldots,n\}$;
\item for each pair of terms $t_1,t_2 \in \terms{\history}$, $[t_1] = [t_2]$ if and
  only if $\rmapext(\bcomp(t_1)) = \rmapext(\bcomp(t_2))$;
\item $\restrict{(\rmapext \circ \bcomp)}{\repset{\H}}$ is an
  isomorphism between  $\db_s(s_s)$ and $\db_c(s_c)$.
\end{enumerate}
We say that $h$ is the \emph{witness of compatibility}. \todo{Should we somehow say that the first three
  conditions guarantee that $\restrict{(\rmapext \circ  \bcomp)}{\repset{\H}}$ is a bijection?}
%
%Notice that
%$\restrict{(\rmapext \circ
%  \bcomp)}{\repset{\H}}$ is guaranteed to be a
%bijection. 
% In fact, by definition different
%representatives belong to distinct equivalence
%classes, and the third condition implies that they are therefore mapped by $\rmapext \circ
%  \bcomp$ to distinct values. 
\todo{We need
  an observation about the fact that
    $\bcomp$ is a bijection. This is guaranteed by construction
  of the symbolic transition systems via representatives (which makes
  also closure under congruence trivially,  vacuously  satisfied).}

\begin{figure*}[t]
\centering
% Everything is drawn on underlying gray rectangles with rounded
% corners.
\tikzstyle{background}=[rectangle, fill=gray!10, inner sep=0.2cm,
rounded corners=5mm]
\begin{tikzpicture}[node distance=5mm,>=latex,text height=1.5ex,text
  depth=0.25ex]

%   \draw[help lines] (0,0) grid (10,10);

 \tikzSimpleState[Rcur,$s_c$,.5,7]; 
\node at (2.5,7) [circle,draw] (Rtemp) {$F_c$}; 
\draw[->] (Rcur) -- node[auto,font=\tiny] {$\doo{}{}{\ldots}$}
 (Rtemp); 
\tikzSimpleState[Rprime,$s^2_c$,9.2,7];
 \draw[->,very thick] (Rtemp) -- (Rprime);
 \tikzSimpleState[Rnext,$s^1_c$,5.5,6];

\tikzSimpleState[Scur,$s_s$,.5,2];
\node at (2.5,2) [circle,draw] (Stemp) {$F_s$};
\draw[->] (Scur) -- node[auto,font=\tiny] {$\doo{}{}{\ldots}$} (Stemp);

\tikzSimpleState[Sprime,$s^1_s$,5.5,3]; 
\draw[->,very thick] (Stemp) -- (Sprime);
\tikzSimpleState[Snext,$s^2_s$,9.2,2];

\pgfarrowsdeclarecombine{dstealth}{dstealth}{stealth}{stealth}{stealth}{stealth}

\node at (0.5,4.5) [rectangle,draw,font=\scriptsize] (BComp) {compatible};
\draw[-] (Scur) -- (BComp);
\draw[-] (BComp) -- (Rcur);

\node at (2.5,4.5) [rectangle,draw,font=\scriptsize] (Iso) {isomorphic};
\draw[-] (Stemp) -- node[auto,font=\scriptsize]
{\em Lemma \ref{lemma:OpenDeterministic-Isomorphism-After-Do}} (Iso);
\draw[-] (Iso) -- (Rtemp);

\node at (6.4,4.5) [rectangle,draw,font=\scriptsize] (BCompExt1) {compatible};
\draw[-] (Sprime) -- node[auto,swap,font=\scriptsize]
{\em Lemma \ref{lemma:OpenDeterministic-Execute-Forth} (2)} (BCompExt1);
\draw[-] (BCompExt1) -- (Rnext);

\node at (10.1,4.5) [rectangle,draw,font=\scriptsize] (BCompExt2) {compatible};
\draw[-] (Snext) -- node[auto,swap,font=\scriptsize]
{\em Lemma \ref{lemma:OpenDeterministic-Execute-Back} (2)} (BCompExt2);
\draw[-] (BCompExt2) -- (Rprime);

\draw[->,very thick,dashed] (Rtemp) -- node[font=\scriptsize] 
{$\begin{array}{l}\\\\\\\textrm{\em Lemma  \ref{lemma:OpenDeterministic-Execute-Forth} (3)}\\\end{array}$} (Rnext);
\draw[->,very thick,dashed] (Stemp) -- node[auto,swap,font=\scriptsize]
{\em Lemma \ref{lemma:OpenDeterministic-Execute-Back} (3)} (Snext);
\draw[->,dotted,thick] (Sprime) -- node[auto,font=\scriptsize] {\em
  Lemma \ref{lemma:OpenDeterministic-Execute-Forth} (1)} (Rnext);
\draw[->,dotted,thick] (Rprime) -- node[auto,swap,font=\scriptsize]
{\emph{Lemma \ref{lemma:OpenDeterministic-Execute-Back} (1)}} (Snext);

   \begin{pgfonlayer}{background}
        \node [background,
                    fit=(Rcur) (Rtemp) (Rprime) (Rnext),
                    label=left:$\cts{\sys}$] {};
         \node [background,
                    fit=(Scur) (Stemp) (Sprime) (Snext),
                    label=left:$\sts{\sys}$] {};
    \end{pgfonlayer}
\end{tikzpicture}
\caption{Intuition behind the proof of history preserving bisimilarity
  between the concrete transition system $\cts{\sys}$ and the symbolic
transition system $\sts{\sys}$ of a \dcds \sys}
\end{figure*}

\begin{lemma} \label{lemma:OpenDeterministic-Isomorphism-After-Do}
Consider a \dcds $\sys = \tup{\dl,\pl}$ with data layer
$\dl=\tup{\CONST, \schema, \EC, \idb}$ and process layer
$\pl=\tup{\FUNC,\aset,\rset}$. Consider the concrete and symbolic
transition systems of $\sys$, respectively defined as $\cts{\sys} =
\tup{\CONST,\schema,\Sigma_c,s^0_c,\db_c,\Longrightarrow_c}$ and $\sts{\sys} =
\tup{\HERBRAND,\schema,\Sigma_s,s^0_s,\db_s,\Longrightarrow_s}$. Given two
compatible states $s_c = \tup{\I_c,\rmap} \in \Sigma_c$ and $s_s =
\tup{\I_s,\history}\in \Sigma_s$ with $h$ witness of the
compatibility, then for every action $\alpha \in \aset$ with
assignment $\sigma$ mapping the parameters of $\alpha$ to values in
$\adom{\I_s}$, there exists a bijection $\bcomp'$ that 
\begin{itemize}
 \item induces an
isomorphism between $F_s = \doo{}{}{\I_s,\alpha\sigma}$ and
$F_c = \doo{}{}{\I_c,\alpha\rmapext(\bcomp(\sigma))}$, and
consequently also between the parameters of the action;
\item is an extension of $\bcomp$ defined as follows: $R(t_1,\ldots,t_n) \in F_s$ if and only if
  $R(\bcomp'(t_1),\ldots,\bcomp'(t_n)) \in F_c$, where for every
  $t_i = f_i(st_1,\ldots,st_m)$, we have that
\end{itemize}
\[
\bcomp'(t_i) = \left\{
\begin{array}{l@{}l}
\bcomp(t_i) &\textrm{ if } t_i \in \domain{\bcomp}\\
f_i(\rmapext(\bcomp(st_1)),\ldots,\rmapext(\bcomp(st_m))) &\textrm{ otherwise}\\
\end{array}
\right.
\]
\end{lemma}
\begin{proof}
The existence of an isomorphism between $F_s$ and $F_c$ is
straightforwardly proven by observing that:
\begin{itemize}
\item  by definition of compatibility, $\restrict{(\rmapext \circ
  \bcomp)}{\repset{\history}}$ is an isomorphism between $\I_s$ and
$\I_c$; 
\item by construction, $\adom{\I_s} \subseteq \repset{\history}$;
\item  the fact that $\restrict{(\rmapext \circ
  \bcomp)}{\repset{\H}}$ is an isomorphism between $\I_s$ and
$\I_c$ implies that $\sigma$ is isomorphic to
$\rmapext(\bcomp(\sigma))$ as well. 
\end{itemize}
We show that $\bcomp'$ is such an isomorphism. Consider an
effect specification $\map{q^+_i\land Q^-_i}{E_i} \in
\effect{\alpha}$. By definition, $E_i$ is a set of facts for
$\schema$, which includes as terms: \myi terms in
$\adom{\idb}$, \myii input parameters, \myiii free variables of $q_i^+$, and  \myiv
terms formed by applying a function $f/N \in \FUNC$ to one of the previous kinds
of terms.
Let us discuss each case separately. By definition, for
each term $d \in \adom{\idb}$ we have that that $d =
\rmapext(\bcomp(d))$. Each input
parameter or free variables of $q_i^+$ in the effect specification is bound by $\doo{}{}{\I_s,\alpha\sigma}$ and
$\doo{}{}{\I_c,\alpha\rmapext(\bcomp(\sigma))}$ to a term
$t \in \adom{\I_s}$ or value $d \in \adom{\I_c}$ respectively, such that $d = \rmapext(\bcomp(t))$. 
Hence, the only case that is not already covered by  $\bcomp$ is the one
in which a function $f/N \in \FUNC$ is applied to one of the previous kinds
of terms. However, it is explicitly managed in the definition of $\bcomp'$.
\end{proof}

\begin{lemma}\label{lemma:OpenDeterministic-Execute-Back}
Consider a \dcds $\sys = \tup{\dl,\pl}$ with data layer
$\dl=\tup{\CONST, \schema, \EC, \idb}$ and process layer
$\pl=\tup{\FUNC,\aset,\rset}$. Consider the concrete and symbolic
transition systems of $\sys$, respectively defined as $\cts{\sys} =
\tup{\CONST,\schema,\Sigma_c,s^0_c,\db_c,\Longrightarrow_c}$ and $\sts{\sys} =
\tup{\HERBRAND,\schema,\Sigma_s,s^0_s,\db_s,\Longrightarrow_s}$. Given two
compatible states $s_c \in \Sigma_c$ and $s_s \in \Sigma_s$, then
for every \cstate $s'_c \in \Sigma_c$ such that $s_c \Longrightarrow_c
s'_c$, there exists an \sstate $s'_s \in \Sigma_s$ such that  $s_s \Longrightarrow_s
s'_s$ and $s'_s$ is compatible with $s'_c$.
\end{lemma}

\begin{proof}
Consider $s_c = \tup{\I_c,\rmap}$, $s'_c  =
\tup{\I'_c,\rmap'}$, $s_s = \tup{\I_s,\history}$, $s'_s  =
\tup{\I'_c,\history'}$, and let $\bcomp$ be the witness of compatibility
between $s_s$ and $s_c$. Consider also $F_s = \doo{}{}{\I_s,\alpha\sigma}$ and
$F_c = \doo{}{}{\I_c,\alpha\rmapext(\bcomp(\sigma))}$, with $\bcomp'$
the extension of $\bcomp$ that
witnesses the isomorphism between $F_s$ and $F_c$, according to Lemma
\ref{lemma:OpenDeterministic-Isomorphism-After-Do}.

The proof is given in three steps:
\begin{description}
\item[Construction of $s'_s$.] We construct $s'_s$ starting
  from $\history$, $F_s$, $\bcomp'$ and $\rmap'$. As a first
  observation, notice that, by definition, $\domain{\rmap'} =
  \image{\bcomp'}$. We define $\history'$ as follows: 
\begin{itemize}
  \item$\history'$ is an
  extension of $\history$;
  \item for each $t_c, t'_c \in
  \domain{\rmap'}$, we have $[h'^{-1}(t_c)]_{\history'} =
  [h'^{-1}(t'_c)]_{\history'}$ if and only if $\rmap'(t_c) =
  \rmap'(t'_c)$;
\item $\repset{\history} \subseteq \repset{\history'}$.
\end{itemize}
Notice that, being $\rmap'$ an extension of $\rmap$,
  the two conditions given for the construction of $\history'$ are
  compatible with each other.
Starting from $F_s$ and
$\history'$, we define $\I'_s = \history'(F_s)$.
\item[$s'_s$ is compatible with $s'_c$.] By construction, $\bcomp'$
satisfies the first two conditions required by
compatibility, and $\history'$ satisfies the third one. Furthermore,
observe that $\history'$ preserves the equality type induced by
$\rmap'$, using $\bcomp'^{-1}$ to connect the service calls in
$\domain{\rmap'}$ with the terms in $s'_s$. Considering that $\bcomp'$
witnesses the isomorphism between $F_s$ and $F_c$, and that
$\history'(F_s)$ replaces each term of $F_s$ with its corresponding
representative in $\history'$, 
$\restrict{(\rmapext' \circ \bcomp')}{\repset{\history'}}$ is an
isomorphism between $\I'_s$ and $\I'_c$. Hence, also the fourth
compatibility condition is met.
\item[$s'_s$ is a successor of $s_s$.] To show that $s_s
  \Longrightarrow_s s'_s$, we prove that
  $\tup{s_s,\alpha\sigma,s'_s} \in  \sexec{\sys}$. In particular:
\begin{enumerate}
\item $\history' = \RCOMM(\I_s,\alpha\sigma,\history)$,
  because $\history'$ extends $\history$ considering all terms
  occurring in $F_s$, and by construction it keeps the previous representatives;
\item by definition, $\I'_s = \history'(\doo{}{}{\I_s,\alpha\sigma})$;
 \item $\I'_s$ satisfies $\EC$, because it is isomorphic to
   $\I'_c$, and $\I'_c$ satisfies $\EC$ by hypothesis. \qed
\end{enumerate}
\end{description}
\end{proof}

\begin{lemma}\label{lemma:OpenDeterministic-Execute-Forth}
Consider a \dcds $\sys = \tup{\dl,\pl}$ with data layer
$\dl=\tup{\CONST, \schema, \EC, \idb}$ and process layer
$\pl=\tup{\FUNC,\aset,\rset}$. Consider the concrete and symbolic
transition systems of $\sys$, respectively defined as $\cts{\sys} =
\tup{\CONST,\schema,\Sigma_c,s^0_c,\db_c,\Longrightarrow_c}$ and $\sts{\sys} =
\tup{\HERBRAND,\schema,\Sigma_s,s^0_s,\db_s,\Longrightarrow_s}$. Given two
compatible states $s_c \in \Sigma_c$ and $s_s \in \Sigma_s$, then
for every \sstate $s'_s \in \Sigma_s$ such that $s_s \Longrightarrow_s
s'_s$, there exists a \cstate $s'_c \in \Sigma_c$ such that  $s_c \Longrightarrow_c
s'_c$ and $s'_s$ is compatible with $s'_c$.
\end{lemma}

\begin{proof}
Consider $s_s = \tup{\I_s,\history}$, $s'_s  =
\tup{\I'_c,\history'}$, $s_c = \tup{\I_c,\rmap}$, $s'_c  =
\tup{\I'_c,\rmap'}$, and let $\bcomp$ be the witness of compatibility
between $s_s$ and $s_c$. Consider also $F_s = \doo{}{}{\I_s,\alpha\sigma}$ and
$F_c = \doo{}{}{\I_c,\alpha\rmapext(\bcomp(\sigma))}$, with $\bcomp'$
the extension of $\bcomp$ that
witnesses the isomorphism between $F_s$ and $F_c$, according to Lemma
\ref{lemma:OpenDeterministic-Isomorphism-After-Do}.

The proof is given in three steps:
\begin{description}
\item[Construction of $s'_c$.] We construct $s'_c$ starting
  from $\rmap$, $F_c$, $\bcomp'$ and $\history'$. As a first
  observation, notice that, by definition, $\terms{\history'} =
  \domain{\bcomp'}$. Let $\repsetc{\history'} = \{t_c \mid
  \textrm{there exists } t_s
  \in \repset{\history'} \textrm{ such that } \bcomp'(t_s) =
  t_c\}$. We define $\rmap'$ as follows:
\begin{itemize}
\item $\rmap':\image{\bcomp'} \rightarrow \CONST$ is an extension of $\rmap$;
\item $\restrict{\rmapext'}{\repsetc{\history'}}$ is a bijection between
  $\repsetc{\history'}$ and $\V$, where $\image{\rmap} \subseteq \V
  \subseteq \CONST$.
\item for every term $t_c \in \domain{\rmap'} \setminus
  \repsetc{\history'}$, we have that $\rmapext'(t_c) = \rmapext'(\bcomp'(\rep{\bcomp'^{-1}(t_c)}{\history'}))$.
\end{itemize}
Starting from $F_c$ and
$\rmap'$, we define $\I'_c = \rmap'(F_c)$.
\item[$s'_c$ is compatible with $s'_s$.] By construction, $\bcomp'$
satisfies the first two conditions required by
compatibility. By construction of $\rmapext'$, we obtain
that:
\begin{itemize}
\item for each representative $r$
that already existed in $\history$, $\rmapext'(\bcomp'(r)) =
\rmapext(\bcomp(r))$;
\item each newly introduced representative is
mapped by $\rmapext' \circ \bcomp'$ to a new value that is different
than all the other ones; 
\item every other term in $\terms{\history'}$ is mapped by $\rmapext' \circ \bcomp'$
to the same value of its representative.
\end{itemize}
Therefore, also the third condition of compatibility is
guaranteed. The last condition of compatibility, which states that
$\restrict{(\rmapext' \circ \bcomp')}{\repset{\history'}}$ is an
isomorphism between $\I'_s$ and $\I'_c$, is guaranteed by construction
of $\rmapext'$, and remembering that by definition $\bcomp'$ witnesses
the isomorphism between $F_s$ and $F_c$.
\item[$s'_c$ is a successor of $s_c$.] To show that $s_c
  \Longrightarrow_c s'_c$, we prove that
  $\tup{s_c,\alpha\rmapext(\bcomp(\sigma),s'_c} \in  \rexec{\sys}$. In particular:
\begin{enumerate}
\item $\rmap' = \RCALLC(\I_c,\alpha\rmapext(\bcomp(\sigma)),\rmap)$,
  because $\rmap'$ extends $\rmap$, and assigns a value to each newly
  introduced service call in $F_c$;
 \item by definition, $\I'_c = \rmap'(\doo{}{}{\I_c,\alpha\rmapext(\bcomp(\sigma))})$;
 \item $\I'_c$ satisfies $\EC$, because $\I'_s$ is isomorphic to
   $\I'_c$, and $\I'_s$ satisfies $\EC$ by hypothesis.\qed
\end{enumerate}
\end{description}
\end{proof}

\begin{lemma}\label{lemma:OpenDeterministic-Extension}
Consider a \dcds $\sys = \tup{\dl,\pl}$ with data layer
$\dl=\tup{\CONST, \schema, \EC, \idb}$ and process layer
$\pl=\tup{\FUNC,\aset,\rset}$. Consider the concrete and symbolic
transition systems of $\sys$, respectively defined as $\cts{\sys} =
\tup{\CONST,\schema,\Sigma_c,s^0_c,\db_c,\Longrightarrow_c}$ and $\sts{\sys} =
\tup{\HERBRAND,\schema,\Sigma_s,s^0_s,\db_s,\Longrightarrow_s}$. Given two
$\cstate$s $s_c,s'_c \in \Sigma_c$ and two $\sstate$s $s_s,s'_s \in
\Sigma_s$ such that:
\begin{itemize}
\item $s_c \Longrightarrow_c s'_c$,
\item $s_s \Longrightarrow_s s'_s$,
\item $s_s$ is compatible with $s_c$, with $\bcomp$ witness of the
  compatibility,
\item $s'_s$ is compatible with $s'_c$, with $\bcomp'$ witness of the
  compatibility,
\end{itemize}
then $\restrict{(\rmapext' \circ \bcomp')}{\repset{\history'}}$ is an
extension of $\restrict{(\rmapext \circ \bcomp)}{\repset{\history}}$.
\end{lemma}
\begin{proof}
The proof is directly obtained by observing that, by definition,
$\rmap'$ is an extension of $\rmap$, $\history'$ is an extension of
$\history$, and $\repset{\history} \subseteq \repset{\history'}$.
\end{proof}

\begin{lemma}
\label{lemma:compatibilityBisimulation}
Consider a \dcds $\sys = \tup{\dl,\pl}$ with data layer
$\dl=\tup{\CONST, \schema, \EC, \idb}$ and process layer
$\pl=\tup{\FUNC,\aset,\rset}$. Consider the concrete and symbolic
transition systems of $\sys$, respectively defined as $\cts{\sys} =
\tup{\CONST,\schema,\Sigma_c,s^0_c,\db_c,\Longrightarrow_c}$ and $\sts{\sys} =
\tup{\HERBRAND,\schema,\Sigma_s,s^0_s,\db_s,\Longrightarrow_s}$. Given two
states $s_s \in \Sigma_s$ and $s_c \in \Sigma_c$, if $s_s$ is
compatible with $s_c$ then $s_s \hbsim s_c$.
\end{lemma}
\begin{proof}
We show that if $s_s = \tup{\I_s,\history}$ is compatible with $s_c = \tup{\I_c,\rmap}$, with $\bcomp$ the
witness of the compatibility, then $s_s \hbsim_{\restrict{(\rmapext \circ
  \bcomp)}{\repset{\history}}} s_c$. In particular, we show that the
three conditions of history preserving bisimulation are guaranteed by
$s_c$, $s_s$ and $\restrict{(\rmapext \circ
  \bcomp)}{\repset{\history}}$:
\begin{enumerate}
   \item  by definition of compatibility, $\restrict{(\rmapext \circ
  \bcomp)}{\repset{\history}}$ is a partial bijection between $\HERBRAND$ and $\CONST$ that induces an isomorphism between $\I_s$ and $\I_c$;
 \item by Lemma \ref{lemma:OpenDeterministic-Execute-Back}, for each
   $s'_c = \tup{\I'_c,\rmap'}$, if $s_c \Longrightarrow_s s'_c$ then there exists
    an $s'_s = \tup{\I'_s,\history'}$ such that $s_s \Longrightarrow_s s'_s$ and $s'_s$ is
    compatible with $s'_c$. Let $\bcomp'$ be the witness of
    compatibility between $s'_s$ and $s'_c$. By Lemma
    \ref{lemma:OpenDeterministic-Extension}, we have that $\restrict{(\rmapext' \circ
  \bcomp')}{\repset{\history'}}$ is an extension of $\restrict{(\rmapext \circ
  \bcomp)}{\repset{\history}}$.
 \item by Lemma \ref{lemma:OpenDeterministic-Execute-Forth}, for each
   $s'_s = \tup{\I'_s,\history}$, if $s_s \Longrightarrow_s s'_s$ then there exists
    an $s'_c = \tup{\I'_c,\rmap'}$ such that $s_c \Longrightarrow_s s'_c$ and $s'_s$ is
    compatible with $s'_c$. Let $\bcomp'$ be the witness of
    compatibility between $s'_s$ and $s'_c$. By Lemma
    \ref{lemma:OpenDeterministic-Extension}, we have that $\restrict{(\rmapext' \circ
  \bcomp')}{\repset{\history'}}$ is an extension of $\restrict{(\rmapext \circ
  \bcomp)}{\repset{\history}}$.\qed
\end{enumerate}
\end{proof}

\begin{theorem}
The concrete and symbolic transition systems of a \dcds \sys are
history preserving bisimilar, i.e., $\sts{\sys} \hbsim \cts{\sys}$.
\end{theorem}
\begin{proof}
Let $\sys = \tup{\dl,\pl}$ be a \dcds with data layer
$\dl=\tup{\CONST, \schema, \EC, \idb}$ and process layer
$\pl=\tup{\FUNC,\aset,\rset}$. Let $\cts{\sys} =
\tup{\CONST,\schema,\Sigma_c,s^0_c,\db_c,\Longrightarrow_c}$ and $\sts{\sys} =
\tup{\HERBRAND,\schema,\Sigma_s,s^0_s,\db_s,\Longrightarrow_s}$.

The proof is straightforwardly obtained from Lemma
\ref{lemma:compatibilityBisimulation} and by noticing that $s^0_s$ is
compatible with $s^0_c$.
\end{proof}

\endinput

%%% Local Variables:
%%% mode: latex
%%% TeX-master: "main"
%%% save-place: t
%%% End:
